# Supplementary material for: Inference after latent variable estimation for single-cell RNA sequencing data
Source: arXiv:2207.00554 source file (2022-10-18)
Supplement: Supplementary file 1 [file appendix_coverage.tex]

\section{Coverage of Confidence Intervals}
\label{appendix_coverage}

We generate data using the mechanism described in Section~\ref{subsec_setup}. For every dataset $\bold{X}$ and each gene $j=1,\ldots,p$, we use the default \texttt{confint.glm}
